# Supplementary material for: Optimal Scheduling for Discounted Age Penalty Minimization in Multi-Loop Networked Control
Source: arXiv:1908.01503 source file (2019-11-22)
Supplement: Supplementary file 1 [file appendix.tex]

\section{First Appendix}
\label{app:A}
